# Supplementary material for: Gate-tunable magnetism of C adatoms on graphene
Source: arXiv:1805.06044 ancillary file (2019-01-09)
Supplement: Supplementary file 1 [file supplemental_material.pdf]

# Supplemental material: Gate-tunable magnetism of C adatoms on graphene

J. Nokelainen[1], I. V. Rozhansky[1,2], B. Barbiellini[1,3], E. Lähderanta[1], and K. Pussi[1]

[1]*LUT University, P.O. Box 20, FI-53851, Lappeenranta, Finland*
[2]*Ioffe Institute, 194021 St. Petersburg, Russia*
[3]*Physics Department, Northeastern University, Boston, Massachusetts 02115, USA*

# 1 Computational details

## 1.1 Precision settings

Tighter support grid for the evaluation of the augmentation charges (`ADDGRID = .TRUE.`) was employed in all of the relaxation calculations. The calculations for the DOS and the total energy were performed fully self-consistently (i.e., without `ICHARG = 11`). In the PBE calculations, we set `PREC = Normal`, but for SCAN more accurate real space grids were used by specifying `PREC = Accurate`. Also `LASPH = .TRUE.` was set for SCAN simulations. Moreover, in the case of SCAN the tolerance of the electronic energy minimization was set to $10^{-5}$ eV and the allowed residual forces were limited to 0.001 eV/Å. These precision settings were used also for PBE in the case of the single adatom on a $4 \times 4$ SC, reported in Sec. III A.

## 1.2 Charging of the system and height of the unit cell

Applying of gate voltage was modeled by altering the electron count in the simulation with the `NELECT` tag. This procedure gives rise to two different error sources. The first one is related to the uniform jellium background charge, which has to be added to the unit cell because the unit cell has to be kept charge neutral due to computational reasons. This background charge spuriously interacts especially with localized states and hence potentially affects total energy, forces and DOS. These errors can be in principle corrected by introducing an appropriate background potential, but its implementation in VASP is only for cubic unit cells and thus cannot be used in our study. However, upon increasing height of the unit cell ($h$) and hence also the unit cell volume, there is a decrease in density of the background charge and thus also in magnitude of the related errors. Thus by using a large vacuum these errors can be overcome. We performed tests for a fully charged ($\Delta Q = 1$) C adatom on a $4 \times 4$ SC with heights $h = 10$ Å and $h = 20$ Å. We obtained nearly

identical DOS and forces in both cases, even though the magnitude of the background charge has a difference by a factor of two in these cases. Thus $h = 20\,\text{Å}$ is enough to avoid all the errors related to the background charge. Therefore $h = 20\,\text{Å}$ has been used as the unit cell height in our work. However, in some high charge cases some charge did escape to the vacuum. The occurrence of this computational issue was found to be proportional to $h$ but inversely proportional to the surface area of the graphene plane. Thus this problem was more significant for smaller SCs and it was necessary to shrink their height. In the case of $6 \times 3$ SCs we used $h = 15\,\text{Å}$ for $\Delta Q \in [1.5\,e,\, 2.0\,e]$ and $h = 13\,\text{Å}$ for charges above $2.0\,e$. In the case of $8 \times 4$ SCs we used $h = 15\,\text{Å}$ for charges above $2.0\,e$ and for the $7 \times 7$ SCs the charge spilling did not occur in the studied $\Delta Q$ range, thus $h = 20\,\text{Å}$ was used in all $7 \times 7$ SC simulations. However, based on the tests we have performed even $h = 13\,\text{Å}$ is enough to avoid all the errors related to the background charge.

Another type of error related to the charging of the system arises from the undesirable spurious electrostatic monopole and dipole interactions induced by the periodic boundary conditions in the $z$ direction, perpendicular to the graphene plane. These effects partly exist also in the case of neutral charge if the system has any dipole moments due to charge transfer. Their effect to the total energy can be corrected and these corrections can be hundreds of electronvolts in magnitude for the charges considered in the present study. However, we use only energy differences $\Delta E = E(\text{FM}) - E(\text{AFM})$ for fixed added charge ($\Delta Q$) and hence the corrections for the FM and AFM solutions mostly cancel each other out. The residual differences in $\Delta E$ were found to be in the meV range. However, taking these differences into account did lead to more noisy but otherwise similar $\Delta E$ curves. Thus, we concluded that these dipole corrections introduce more error than corrections to $\Delta E$ and decided to neglect them.

## 1.3 Conventional RKKY regime

In the conventional RKKY region, numerical instability is always present, leading to significantly slower electronic and structural convergence. The numerical instability is most evident in the AFM solution but it is also present in lesser extent in the FM solution. The instability is stronger for smaller magnetizations. In fact, the structural convergence within the tight convergence criterion of $0.001\,\text{eV/Å}$ was not reached for the smallest studied $\Delta Q$ values for $\beta(6 \times 3)$ and $\gamma(6 \times 3)$, but the final forces were not larger than few $0.001\,\text{eV/Å}$. Thus the structural error was in the range of $0.001\,\text{Å}$. In these cases, the observed AFM values of $E_{\text{ex}}^{\text{conv}}$ were strong, namely 104 meV, 76 meV and 115 meV for $\beta(\overline{\Delta Q} = -0.25\,e)$, $\gamma(-0.25\,e)$ and $\gamma(-0.5\,e)$, respectively. Thus the tiny structural errors in these cases do not significance affect these results. Moreover, the structural relaxation is performed with lesser computational accuracy than the final total energy calculations. Therefore, some forces appear in the total energy calculations. For example, in the case of $\beta(6 \times 3)$, the total energy calculation of the AFM solution gives forces a bit larger than $0.01\,\text{eV/Å}$ on the adatoms, which is larger than the above force error related to structural relaxations.

As discussed in the main text, the expected low-magnetization AFM peak of the $\alpha(8 \times 4)$ array related to conventional RKKY was not confirmed, but this does not invalidate our results. The first reason is that the nature of the $E_{\text{ex,bri}}^{\text{conv}}$ energy term in Eq. (4) is based on approximation of summing $AA$ and $AB$-type interactions together, and these interactions also contain competing

FM and AFM interactions. Therefore, the prediction of the small AFM peak might not be correct. The second reason is that the discussed numerical instability in the conventional RKKY region can play a role. In fact, $\Delta E$ was found to be sensitive to the computational details such as the density of the real-space grids and the amount of $k$-points. This behavior was observed despite the fact that the electronic convergence was reached in all calculations. This trend reveals a complex energy landscape in the conventional RKKY region. Therefore, numerical error in the meV scale might still be present in the lowest magnetization values for the SCAN simulations. As a matter of fact, we observed an AFM peak with lesser computational precision, but this feature disappeared when the computational accuracy was increased.

## 2 Energetics of the two-adatom configurations

We found in accordance with the previous literature that in dimerization process of the adatoms the second adatom climbs on top the first adatom, and the adatom pair loses all the magnetization and migrates on a top site on the graphene sheet. The dimer was found to have 5.42 eV lower energy than the Conf. #4 ($7 \times 7$ SCs were used), which has the lowest total energy among the one-sided adsorption cases. We also calculated the energy of a single adatom on a $7 \times 7$ SC, and obtained with formula $E_{\text{dimer}} + E_{\text{clean graphene}} - 2 \cdot E_{\text{adatom}}$ that two bridge-site adatoms have 5.73 eV higher energy than the dimerized solution. Based on this there is an energy gain of 314 meV when two adatoms far away from each other is taken to the close interaction Conf. #4, which indicates the existence of strong attractive potential between the adatoms due to the high energy gain by dimerization. Most of this energy is gained due to the fact that the structural distortions of the graphene sheet are partially shared by the adatoms (the structural distortions are strong, as discussed in the main text Sec. III A). However, we emphasize that the Conf. #4 is still metastable, but low temperatures are required for its stabilization.

**Table 1:** Total energy of each adatom pair configuration (i): with respect to the dimer solution computed at $7 \times 7$ SC. (ii – in parenthesis): with respect to $7 \times 7$ Conf. #4, which has the lowest total energy among the one-sided adsorption cases.

| | Relative total energy (eV) | | |
|---|---|---|---|
| Conf. | $7 \times 7$ | $7 \times 7$ (two-sided) | $6 \times 3$ |
| #1 | 5.60 (+0.183) | 5.40 (−0.016) | 5.64 (+0.227) |
| #2 | 5.56 (+0.139) | 5.55 (+0.129) | 5.70 (+0.288) |
| #3 | 5.61 (+0.196) | 5.61 (+0.191) | 5.75 (+0.330) |
| #4 | 5.42 (+0.000) | 5.38 (−0.035) | 5.48 (+0.063) |
| #5 | 5.54 (+0.125) | 5.54 (+0.128) | 5.63 (+0.217) |
| #6 | 5.75 (+0.337) | 5.68 (+0.260) | 5.75 (+0.335) |
| #7 | 5.65 (+0.233) | 5.65 (+0.229) | 5.70 (+0.278) |
| #8 | 5.63 (+0.217) | 5.58 (+0.167) | 5.71 (+0.294) |

Table 1 contains the total energies of each adatom pair configuration #1 – #8. The energies have been given in relation to the $7 \times 7$ SC dimer solution and also to the Conf. #4. Also the $6 \times 3$ SC

sizes are considered. In these cases the $7 \times 7$ SC dimer and Conf. #4 results have been converted to $6 \times 3$ SC by subtracting the primitive cell energy ($-4.543\,\mathrm{eV}$) $7 \cdot 7 - 6 \cdot 3 = 31$ times from them.

Interestingly, the Conf. #4 has the lowest energy within both SC sizes and for both one-sided and two-sided adsorptions. This might be due to low symmetry of this configuration, which allows symmetric displacements of the graphene atoms. In accordance with this possible explanation also another high-symmetry configuration (Conf. #5) is rather low in energy. Apart from that, the adatom pairs with lower separations (Confs. #1 – #3) are lower in energy than the adatom pairs with higher separations (Confs. #6 – #8). This behavior is due to the attractive potential between the adatoms, and enhances the dimerization of the adatoms. The two-sided configuration is energetically more favorable in nearly every case, which is most likely due to smaller amount of curvature-related bending energy on the graphene sheet. Most likely for the same reason nearly all configurations have a higher energy when placed on a $6 \times 3$ SC than on a $7 \times 7$ SC.

Table 2 contains the total energies of each adatom array configuration. The energies are again in relation to the $7 \times 7$ SC dimer structure and $7 \times 7$ SC Conf. #4. Scaling the results to $7 \times 7$ SC size have been done similarly as for the close interaction pairs above. Each case is clearly higher in energy than the $7 \times 7$ SC Conf. #4. In each case the two-sided adsorption energies are lower than the corresponding one-sided adsorption energies and each configuration nearly always has lower energy on the larger SC. These two observations are in accordance with the close interaction pair results. The $\gamma$ array yields the lowest total energy in every SC type, which is in accordance with the strong stabilization of the FM solution in each case.

**Table 2:** Total energy of each adatom array configuration (i): with respect to the dimer solution computed at $7 \times 7$ SC. (ii – in parenthesis): with respect to $7 \times 7$ Conf. #4, which has the lowest total energy among the one-sided adsorption close interaction pairs.

| | Relative total energy (eV) | | | |
|---|---|---|---|---|
| Conf. | $6 \times 3$ | $6 \times 3$ (two-sided) | $8 \times 4$ | $8 \times 4$ (two-sided) |
| $\alpha$ | 5.88 (+0.460) | 5.72 (+0.299) | 5.75 (+0.330) | 5.66 (+0.243) |
| $\beta$ | 5.85 (+0.435) | 5.67 (+0.253) | 5.73 (+0.314) | 5.65 (+0.232) |
| $\gamma$ | 5.77 (+0.349) | 5.62 (+0.199) | 5.72 (+0.305) | 5.64 (+0.222) |

# 3 Remarks on the close interaction pair configurations

## 3.1 The effects of periodicity at the $7 \times 7$ SCs

We have taken several approaches to estimate the significance of periodicity-induced effects on the $7 \times 7$ SC close interaction pairs. In the case of the $7 \times 7$ SCs the range of adatom separations is between 3.7 Å (Conf. #1) and 5.7 Å (Conf. #8). The range of adatom separations in neighbouring unit cells (between periodic images) is between 11.7 Å (Conf. #8) and 13.6 Å (Conf. #1). Fig. 1 illustrates the situation for the Conf. #8. The question is if the interactions between the periodic adatom images are sufficiently small when compared to the pairwise interactions of the two adatoms

within the unit cell. As explained below, we conclude that this is the case (with a maximum 3–4 meV contribution from the periodic effects).

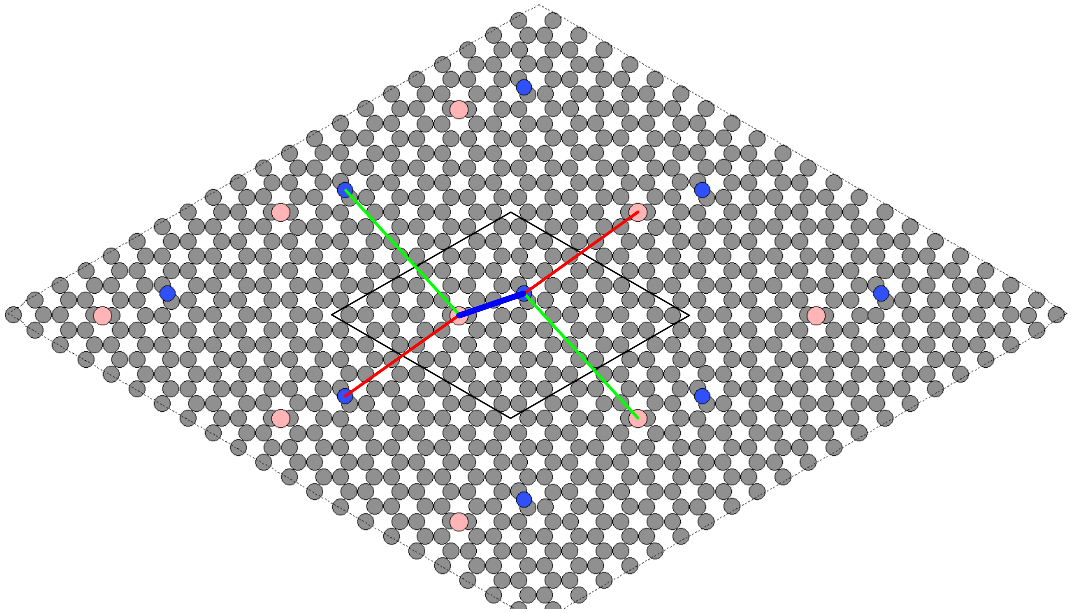

**Figure 1:** Conf. #8 on a $7 \times 7$ SC (black lines). $C_1^{ad}$ and $C_2^{ad}$ are colored in blue and blush, respectively. The short-range interaction between the adatoms (5.7 Å) is colored in blue. The nearest-neighbor interactions between periodic images (11.7 Å) are denoted in red. There exists one such interaction per unit cell. The next-nearest-neighbor interactions between periodic images (14.2 Å) are denoted in green. There exists one such interaction per unit cell.

First of all, as discussed in the section for single adatoms on $N \times N$ SCs (Sec. III A), the width of the DOS impurity peak is related to the magnitude of the hybridization between its periodic images, and it has the following trend for different SCs: $3 \times 3$: 0.23 eV; $4 \times 4$: 0.10 eV; $5 \times 5$: 0.08 eV; $6 \times 6$: 0.04 eV; $7 \times 7$: 0.03 eV; $9 \times 9$: 0.03 eV; $9 \times 9$: 0.02 eV. The case $N = 5$ corresponds to adatom separation of 12.3Å, which is close to the interaction distance between periodic images in the case of Conf. #8. At this value the peak width is not converged, but it is already small, so the isolation of the adatom pair can be considered to be reasonably good, even though it is not perfect.

Secondly, as discussed in Sec. III C in the main text as well as in the next subsection of this document, in the close interaction pair configurations the adatom-adatom interactions are strong enough to severely deform the electronic structure of the adatoms and the Dirac cone of graphene. This is the case for all the pair configurations, even for Conf. #8. The DOS effects of the interactions between periodic adatom images can be estimated from the results on single adatoms on $N \times N$ SCs and remote interaction array results. These results show that the interactions are only able to create a small broadening to the DOS peaks associated with the $\psi_{p,\perp}$ state for interaction distances higher than 10 Å. Since the separations between the periodic images are at least 11.7 Å for the close interaction pairs at $7 \times 7$ SCs, the interactions between the adatom pairs within the SC are much stronger than between the periodic images.

Thirdly, the adatom arrays (discussed in the main text Sec. III B) can be used to estimate the

magnitudes of the remote interactions. In the case of the $8 \times 4$ SC arrays the maximums of $\Delta E$ are in the range of $2-20$ meV, depending on the configuration. The adatom separations are in the range of $8.9-9.9$ Å in these cases (the highest $\Delta E$ values and smallest separations are obtained for the $\gamma$ array). There exists six adatom-adatom pairs per one computational unit cell, as illustrated in the main text Fig. 2 (a),[1] thus the $\Delta E$ associated to one adatom-adatom pair is at maximum $3-4$ meV for the adatom separation range of $8.9-9.9$ Å. In the case of the the adatom pairs, there exists only one nearest-neighbor interaction pair per one computational unit cell, as illustrated in Fig. 1, and this interaction pair is expected to contain majority of the periodicity-induced effects. Based on the above considerations the $\Delta E$ associated to this pair would be at maximum $3-4$ meV if the interaction distance was in the range of $8.9-9.9$ Å, but in fact it is even larger (11.7 Å for Conf. #8 and more for others).

Fourthly, we have also studied the close interaction pairs on $6 \times 3$ SCs in our work in order to examine the effect of strong interactions between the periodic images of the adatoms. However, our results on these small SCs were very similar to the $7 \times 7$ SC results. This shows that the observed effects in the close interaction pair configurations are not periodicity-induced, instead all the physics are contained in the pairwise interaction between the adatoms.

Fifthly, the adatom-adatom interactions are expected to decay rapidly as a function of the adatom separation. The RKKY interactions are proportional to $1/r^3$ and the $\psi_{p,\perp}$ wavefunctions decay exponentially. Since the separation ratios of the short-range pairwise interactions and the interactions between the periodic images are in the range of $2.0-3.7$ for the $7 \times 7$ SC close interaction cases, the pairwise interactions are always significantly larger than the interactions between the periodic images.

All the above points should demonstrate that the studied adatom pairs are reasonably well isolated when placed on $7 \times 7$ SCs.

Lastly we would like to note that in this case it is not reliable to inspect the periodicity-induced effects by studying the energies of the pair configurations with the SC size as the variable, as one would proceed in the usual cases. In our case different SC size leads to different adatom density, which means that individual adatom receives different portion of the charge transfer from graphene. Our results in general show that the energetic and magnetic properties of the C adatoms are sensitive to the charge differences ($\Delta Q$). Moreover, the energy related to curvature of the graphene sheet is not constant for different SC sizes.

## 3.2 Magnetic moments of the adatoms

As discussed in the main text, in the case of close interaction pairs the magnetization curves of the close interaction configurations display peculiar nonlinear behavior (see particularly the main text Fig. 6). This mechanism originates from the fact that the $\psi_{p,\parallel}$ orbitals also play a role below $\overline{\Delta Q} = 0.5\, e$ since their energies have been lifted to $E_{\mathrm{F}}$ due to strong interactions between adatoms

[1] The weight of each adatom-adatom interaction that extends to the neighbouring unit cell has to be divided by two.

**Table 3:** Summary for which $\overline{\Delta Q}$ values the FM and AFM solutions are *not* well-defined and why. For example when lowering $\overline{\Delta Q}$ to such values, the FM solution might become FIM (FM $\to$ FIM). Sometimes only one stable solution in the system, which can occur if for example the AFM solution becomes FM (AFM $\to$ FM) or both FM and AFM solutions become FIM (AFM, FM $\to$ FIM).

| Conf. | $7 \times 7$ | $7 \times 7$ (two-sided) | $6 \times 3$ |
|---|---|---|---|
| #1 | $\leq 0.25\,e$: FM $\to$ FIM | | $= 0.25\,e$: AFM $\to$ FIM |
| #2 | | $\leq 0\,e$: AFM $\to$ FIM | $\leq 0.25\,e$: AFM $\to$ FIM |
| #3 | $\leq -0.75\,e$: AFM, FM $\to$ FIM | $\leq -0.5\,e$: AFM $\to$ FM | $\leq 0.25\,e$: AFM $\to$ FIM |
| #4 | | | |
| #5 | | | |
| #6 | $\leq -0.75\,e$: AFM $\to$ FIM | | |
| #7 | $\leq -0.5\,e$: AFM $\to$ FIM | $\leq 0.5\,e$: AFM $\to$ FIM | $\leq -0.25\,e$: AFM $\to$ FIM |
| #8 | $\leq -0.25\,e$: AFM, FM $\to$ FIM | $\leq -0.25\,e$: AFM $\to$ FM | |

and large structural distortions. Moreover, due to this mechanism the magnetic moments of $C_1^{ad}$ and $C_2^{ad}$ (labeled as $M_1$ and $M_2$, respectively) become different in magnitude in many cases. This causes the AFM solution to become ferrimagnetic (FIM) solution with nonzero total magnetization. This occurs for example for Conf. #7 with any studied SC. Sometimes there is only one stable ferrimagnetic solution in the system. This happens for example for Conf. #8 ($7 \times 7$ SC) below $\overline{\Delta} = -0.25\,e$. Table 3 summarizes for which configurations and $\overline{\Delta Q}$ values these anomalies occur in the studied range. In general the behaviors between different SC sizes are similar. Interestingly, the behavior of Conf. #1 varies significantly on different SCs. In the $7 \times 7$ SC with two-sided adsorption, the FM and AFM solutions of Conf. #1 are always defined. In the $6 \times 3$ SC, the FM solution is always defined, and the AFM solution becomes FIM only for $\overline{\Delta Q} = 0.25\,e$. Also in the $7 \times 7$ SC with one-sided adsorption the AFM solution becomes FIM only for $\overline{\Delta Q} = 0.25\,e$. However, in this SC the FM solution becomes FIM for $\overline{\Delta Q} \leq 0.25\,e$, therefore solutions with parallel spins were not found for most of the $\Delta E$ curve.

The smallest studied $\overline{\Delta Q}$ values were $-0.75\,e$ for $7 \times 7$ and $-0.5\,e$ for $6 \times 3$ SCs. In some cases (for example in the two-sided adsorption version of Conf. #6), the adatoms still have large magnetic moments even at these $\overline{\Delta Q}$ values due to the $\psi_{p,\parallel}$ states, but the FM and AFM solutions are still well-defined. However, we do not know if this is still the case if even more electrons were further removed from the system.

As an detailed example we consider Conf. #7, for which magnetization decreases when more charge is added in the range of $\overline{\Delta Q} \in [-0.25\,e, 0.25\,e]$ (as is evident from Fig. 6 in the main text). We present PDOS plots of Conf. #7 projected to $C_1^{ad}$ and $C_2^{ad}$ at $\overline{\Delta Q} = 0$ in Figs. 2 (a) and (b), respectively. In this particular case, only the $\psi_{p,\perp;\uparrow}$ state of $C_2^{ad}$ (at $E_F$) and the $\psi_{p,\parallel;\downarrow}$ states of both adatoms (between $-0.04$ eV and $0.20$ eV) remain well-defined. The rest of the states experience some hybridization with each other and the states of the basal atoms. As a result there is an unoccupied spin up orbital between $0.10$ eV and $0.21$ eV. Partial charge density visualization reveals that it is related to the $\psi_{p,\perp;\uparrow}$ and $\psi_{p,\parallel;\uparrow}$ states of $C_1^{ad}$. According to the partial charge analysis, the occupied state between $-0.33$ eV and $-0.10$ eV are related to the $\psi_{p,\perp;\uparrow}$ states of the both adatoms. Nevertheless, despite of the complexity of the situation, the DOS plot helps to

understand the reason why the magnetization decreases when more charge is added. The $\psi_{p,\parallel;\downarrow}$ states are partly occupied with high PDOS, and adding charge occupies these minority spin states. Once these states are filled, the complex situation simplifies and the $\psi_{p,\perp}$ and $\psi_{p,\parallel}$ states of both adatoms become well-defined again.

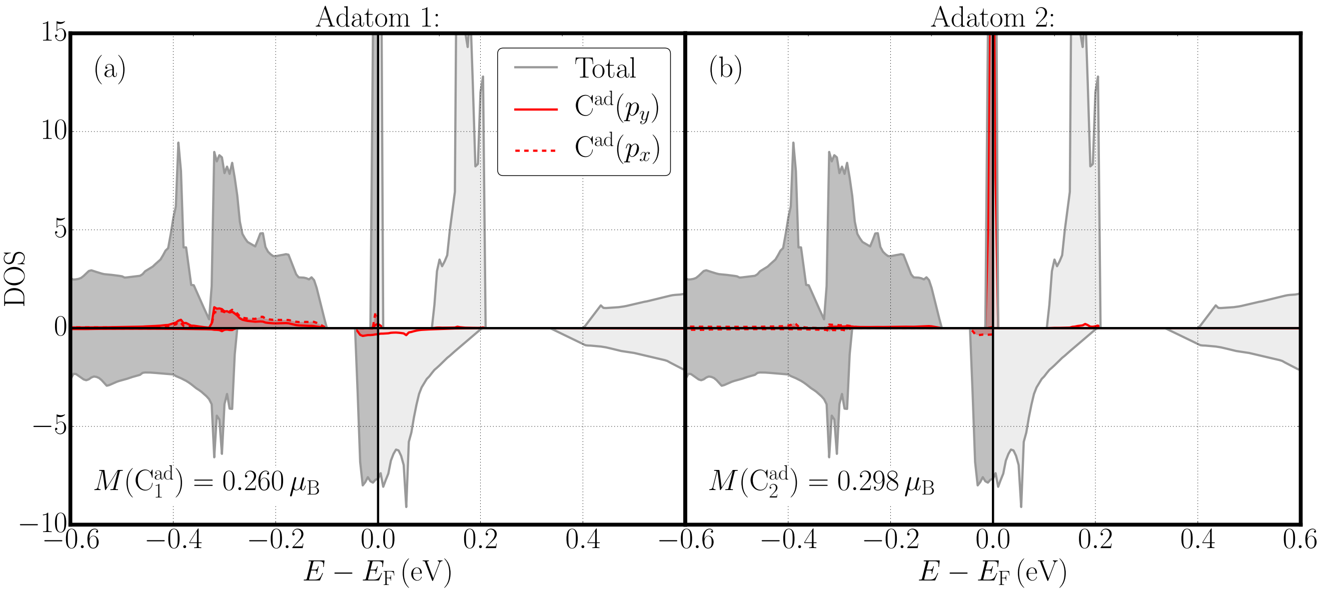


**Figure 2:** PDOS plots of Conf. #7 (neutral charge) projected to both (a) $C_1^{ad}$ and (b) $C_2^{ad}$.
